# Supplementary material for: Maintenance of Strongly Connected Component in Shared-memory Graph
Source: arXiv:1804.01276 source file (2018-04-10)
Supplement: Supplementary file 1 [file appendix.tex]

\begin{center}
\Large\textbf{Appendix}
\end{center}
All the details missing from the main text are mentioned here. 
\input{app-model}
\input{app-conc-graph}
\input{app-working}
\input{app-correctness}
\input{app-acyclicty}
%\section{Data-Structure Specific Proofs}
%\input{app-ds-proof}
